# Supplementary material for: vdW-DF Study of energetic, structural, and vibrational properties of small water clusters and ice Ih
Source: arXiv:1106.4830 ancillary file (2011-06-23)
Supplement: Supplementary file 1 [file Kolb_Thonhauser_supplemental.pdf]

# Supplemental material: vdW-DF study of energetic, structural, and vibrational properties of small water clusters and ice $I_h$

Brian Kolb and T. Thonhauser
*Department of Physics, Wake Forest University, Winston-Salem, NC, 27109*
(Dated: June 23, 2011)

## ATOMIC COORDINATES

Fully relaxed (as described in the main text) Cartesian coordinates for each system and method are given in the following tables as $x, y, z$ triplets in Angstrom (Å).

### Monomer Coordinates

| | LDA | | | PBE | | | vdW-DF | | | MP2 | | |
|---|---|---|---|---|---|---|---|---|---|---|---|---|
| | $x$ | $y$ | $z$ | $x$ | $y$ | $z$ | $x$ | $y$ | $z$ | $x$ | $y$ | $z$ |
| O | 0.0000 | 0.0000 | −0.0017 | 0.0000 | 0.0000 | 0.0015 | 0.0000 | 0.0000 | 0.0039 | 0.0000 | 0.0000 | 0.0046 |
| H | 0.0000 | 0.7760 | 0.5988 | 0.0000 | 0.7713 | 0.5972 | 0.0000 | 0.7719 | 0.5961 | 0.0000 | 0.7581 | 0.5957 |
| H | 0.0000 | −0.7760 | 0.5988 | 0.0000 | −0.7713 | 0.5972 | 0.0000 | −0.7719 | 0.5961 | 0.0000 | −0.7581 | 0.5957 |

### Dimer Coordinates

| | LDA | | | PBE | | | vdW-DF | | | MP2 | | |
|---|---|---|---|---|---|---|---|---|---|---|---|---|
| | $x$ | $y$ | $z$ | $x$ | $y$ | $z$ | $x$ | $y$ | $z$ | $x$ | $y$ | $z$ |
| O | 0.0000 | 0.1246 | −0.0440 | 0.0000 | 0.0251 | 0.0078 | 0.0000 | −0.0507 | 0.0303 | 0.0000 | −0.0159 | 0.0224 |
| H | 0.0000 | −0.2732 | 0.8514 | 0.0000 | −0.3111 | 0.9211 | 0.0000 | −0.3832 | 0.9437 | 0.0000 | −0.3312 | 0.9296 |
| H | 0.0000 | 1.1133 | 0.1048 | 0.0000 | 1.0066 | 0.0947 | 0.0000 | 0.9248 | 0.1092 | 0.0000 | 0.9491 | 0.1022 |
| O | 0.0000 | 2.8400 | 0.0595 | 0.0000 | 2.8935 | 0.0041 | 0.0000 | 2.9544 | −0.0272 | 0.0000 | 2.9163 | −0.0189 |
| H | 0.7813 | 3.1017 | −0.4758 | 0.7751 | 3.1970 | −0.5037 | 0.7745 | 3.2813 | −0.5179 | 0.7609 | 3.2449 | −0.5076 |
| H | −0.7813 | 3.1017 | −0.4758 | −0.7751 | 3.1970 | −0.5037 | −0.7745 | 3.2813 | −0.5179 | −0.7609 | 3.2449 | −0.5076 |

### Trimer Coordinates

| | LDA | | | PBE | | | vdW-DF | | | MP2 | | |
|---|---|---|---|---|---|---|---|---|---|---|---|---|
| | $x$ | $y$ | $z$ | $x$ | $y$ | $z$ | $x$ | $y$ | $z$ | $x$ | $y$ | $z$ |
| O | −0.1848 | 1.4533 | 0.1681 | −0.1679 | 1.5533 | 0.1305 | −0.1972 | 1.6330 | 0.1179 | −0.2062 | 1.5976 | 0.1126 |
| H | 0.6425 | 0.8536 | 0.0864 | 0.6388 | 0.9742 | 0.0529 | 0.6261 | 1.0954 | 0.0790 | 0.6097 | 1.0675 | 0.0745 |
| H | −0.1456 | 2.1024 | −0.5658 | −0.1256 | 2.1807 | −0.6129 | −0.1241 | 2.2911 | −0.5939 | −0.1114 | 2.2569 | −0.5799 |
| O | 1.3731 | −0.5726 | −0.0962 | 1.4471 | −0.6364 | −0.1141 | 1.5285 | −0.6463 | −0.0569 | 1.5002 | −0.6227 | −0.0558 |
| H | 1.8720 | −0.9439 | 0.6615 | 1.9628 | −1.0105 | 0.6219 | 2.0916 | −1.0734 | 0.6101 | 2.0583 | −1.0622 | 0.5907 |
| H | 0.4412 | −0.9973 | −0.0871 | 0.5474 | −1.0598 | −0.0719 | 0.6635 | −1.1133 | −0.0315 | 0.6450 | −1.0855 | −0.0188 |
| O | −1.1767 | −0.8896 | −0.1929 | −1.2729 | −0.9315 | −0.1265 | −1.3255 | −0.9907 | −0.1340 | −1.2858 | −0.9832 | −0.1214 |
| H | −1.7530 | −1.2198 | 0.5280 | −1.8569 | −1.2187 | 0.5973 | −1.9948 | −1.2781 | 0.5092 | −1.9747 | −1.2486 | 0.4930 |
| H | −1.0644 | 0.1199 | −0.0530 | −1.1686 | 0.0544 | −0.0283 | −1.2639 | −0.0119 | −0.0509 | −1.2308 | −0.0138 | −0.0459 |

**Tetramer Coordinates**

| | LDA | | | PBE | | | vdW-DF | | | MP2 | | |
|---|---|---|---|---|---|---|---|---|---|---|---|---|
| | $x$ | $y$ | $z$ | $x$ | $y$ | $z$ | $x$ | $y$ | $z$ | $x$ | $y$ | $z$ |
| O | 0.2097 | −1.7679 | −0.0194 | 0.1980 | −1.8732 | −0.0289 | 0.2072 | −1.9594 | 0.0227 | 0.2134 | −1.9366 | 0.0135 |
| H | −0.6849 | −1.2159 | −0.0070 | −0.6610 | −1.3444 | −0.0127 | −0.6465 | −1.4554 | −0.0007 | −0.6322 | −1.4411 | −0.0054 |
| H | 0.2086 | −2.3487 | 0.7702 | 0.1674 | −2.4715 | 0.7381 | 0.1485 | −2.5619 | 0.7830 | 0.1362 | −2.5411 | 0.7562 |
| O | 1.2159 | −0.6849 | 0.0070 | 1.3444 | −0.6610 | 0.0127 | 1.4554 | −0.6465 | 0.0007 | 1.9366 | 0.2134 | −0.0135 |
| H | 1.7679 | 0.2097 | 0.0194 | 1.8732 | 0.1980 | 0.0289 | 1.9594 | 0.2072 | −0.0227 | 2.5411 | 0.1362 | −0.7562 |
| H | 2.3488 | 0.2086 | −0.7702 | 2.4715 | 0.1674 | −0.7381 | 2.5619 | 0.1485 | −0.7830 | 1.4411 | −0.6322 | 0.0053 |
| O | −1.7679 | −0.2097 | 0.0194 | −1.8732 | −0.1980 | 0.0289 | −1.9594 | −0.2072 | −0.0227 | −1.9366 | −0.2134 | −0.0135 |
| H | −2.3488 | −0.2086 | −0.7701 | −2.4716 | −0.1674 | −0.7381 | −2.5619 | −0.1485 | −0.7829 | −2.5411 | −0.1362 | −0.7562 |
| H | −1.2159 | 0.6849 | 0.0070 | −1.3444 | 0.6610 | 0.0127 | −1.4554 | 0.6465 | 0.0007 | −1.4411 | 0.6322 | 0.0053 |
| O | −0.2097 | 1.7679 | −0.0194 | −0.1980 | 1.8732 | −0.0289 | −0.2072 | 1.9594 | 0.0227 | −0.2134 | 1.9366 | 0.0135 |
| H | −0.2086 | 2.3487 | 0.7702 | −0.1674 | 2.4715 | 0.7381 | −0.1485 | 2.5619 | 0.7830 | −0.1362 | 2.5411 | 0.7562 |
| H | 0.6849 | 1.2159 | −0.0070 | 0.6610 | 1.3444 | −0.0127 | 0.6465 | 1.4554 | −0.0007 | 0.6322 | 1.4411 | −0.0053 |

**Pentamer Coordinates**

| | LDA | | | PBE | | | vdW-DF | | | MP2 | | |
|---|---|---|---|---|---|---|---|---|---|---|---|---|
| | $x$ | $y$ | $z$ | $x$ | $y$ | $z$ | $x$ | $y$ | $z$ | $x$ | $y$ | $z$ |
| O | −0.5658 | 2.0460 | −0.1214 | −0.5499 | 2.1843 | −0.0570 | −0.5280 | 2.2883 | −0.0525 | −0.5376 | 2.2562 | −0.0883 |
| O | 1.7717 | 1.1609 | −0.0614 | 1.9003 | 1.1921 | −0.0693 | 2.0143 | 1.1997 | −0.1198 | −0.5134 | 3.0349 | 0.4733 |
| O | 1.6543 | −1.3273 | 0.1370 | 1.7257 | −1.4391 | 0.1134 | 1.7697 | −1.5387 | 0.1892 | 0.3835 | 1.9160 | −0.0953 |
| O | −0.7466 | −1.9889 | −0.0657 | −0.8302 | −2.0861 | −0.0523 | −0.9056 | −2.1649 | −0.1208 | 1.9894 | 1.1953 | −0.0891 |
| O | −2.1309 | 0.0927 | −0.0050 | −2.2484 | 0.1449 | −0.0401 | −2.3483 | 0.1907 | 0.0266 | 1.9515 | 0.2223 | 0.0364 |
| H | −0.6468 | 2.7456 | 0.5595 | −0.5835 | 2.8646 | 0.6375 | −0.5164 | 3.0322 | 0.5722 | 2.5396 | 1.3227 | −0.8664 |
| H | 2.2835 | 1.3695 | −0.8708 | 2.4214 | 1.3864 | −0.8679 | 2.5450 | 1.3459 | −0.9209 | 1.7529 | −1.5179 | 0.1938 |
| H | 2.0044 | −1.6886 | 0.9778 | 2.0748 | −1.8365 | 0.9301 | 2.0768 | −1.9577 | 1.0104 | 0.8185 | −1.7906 | 0.0649 |
| H | −0.9560 | −2.4721 | −0.8922 | −1.0812 | −2.5783 | −0.8533 | −1.1788 | −2.6188 | −0.9356 | 2.0389 | −1.9681 | 0.9926 |
| H | −2.7010 | 0.1448 | 0.7901 | −2.8728 | 0.2366 | 0.7003 | −2.9734 | 0.3115 | 0.7605 | −0.8897 | −2.1420 | −0.1519 |
| H | 0.4348 | 1.6978 | −0.0967 | 0.3998 | 1.8339 | −0.0648 | 0.4003 | 1.9354 | −0.0811 | −1.1779 | −2.5652 | −0.9647 |
| H | 1.7538 | 0.1055 | 0.0325 | 1.8691 | 0.1833 | 0.0093 | 1.9717 | 0.2151 | 0.0058 | −1.4422 | −1.3342 | −0.0742 |
| H | 0.6455 | −1.6404 | 0.0514 | 0.7557 | −1.7221 | 0.0499 | 0.8203 | −1.8095 | 0.0770 | −2.3318 | 0.1772 | 0.0668 |
| H | −1.3552 | −1.1223 | −0.0437 | −1.3982 | −1.2483 | −0.0455 | −1.4586 | −1.3416 | −0.0648 | −2.8972 | 0.3003 | 0.8333 |
| H | −1.5079 | 0.9479 | −0.0137 | −1.6447 | 0.9554 | −0.0124 | −1.7513 | 0.9836 | 0.0317 | −1.7468 | 0.9643 | 0.0467 |

**Ice $I_h$ Coordinates**

| | LDA | | | PBE | | | vdW-DF | | |
|---|---|---|---|---|---|---|---|---|---|
| | $x$ | $y$ | $z$ | $x$ | $y$ | $z$ | $x$ | $y$ | $z$ |
| H | 0.3344 | 0.0000 | 0.2152 | 2.5392 | 0.0000 | 1.4559 | 2.6442 | 0.0070 | 1.4814 |
| H | 0.6656 | 0.0000 | 0.7152 | 5.0363 | 0.0000 | 5.0293 | 5.1917 | 0.0062 | 5.1606 |
| H | 0.6656 | 0.6656 | 0.2152 | 2.5181 | 4.3616 | 1.4559 | 2.5958 | 4.4961 | 1.4845 |
| H | 0.3344 | 0.3344 | 0.7152 | 1.2696 | 2.1990 | 5.0293 | 1.3216 | 2.2890 | 5.1612 |
| H | 0.0000 | 0.3344 | 0.2152 | −1.2696 | 2.1990 | 1.4559 | −1.3160 | 2.2934 | 1.4814 |
| H | 0.0000 | 0.6656 | 0.7152 | −2.5181 | 4.3616 | 5.0293 | −2.5905 | 4.4993 | 5.1606 |
| H | 0.4728 | 0.0000 | 0.0097 | 3.4810 | 0.0000 | 0.1335 | 3.5734 | 0.0057 | 0.1798 |
| H | 0.5272 | 0.0000 | 0.5097 | 4.0945 | 0.0000 | 3.7069 | 4.2620 | 0.0071 | 3.8589 |
| H | 0.5272 | 0.5272 | 0.0097 | 2.0472 | 3.5459 | 0.1335 | 2.1308 | 3.6907 | 0.1826 |
| H | 0.4728 | 0.4728 | 0.5097 | 1.7405 | 3.0146 | 3.7069 | 1.7866 | 3.0945 | 3.8602 |
| H | 0.0000 | 0.4728 | 0.0097 | −1.7405 | 3.0146 | 0.1335 | −1.7818 | 3.0976 | 0.1798 |
| H | 0.0000 | 0.5272 | 0.5097 | −2.0472 | 3.5459 | 3.7069 | −2.1248 | 3.6945 | 3.8589 |
| H | 0.8053 | 0.1376 | 0.9876 | 5.5318 | 0.8132 | 7.0456 | 5.7179 | 0.8052 | 7.2699 |
| H | 0.3323 | 0.1376 | 0.4876 | 2.0437 | 0.8132 | 3.4722 | 2.1202 | 0.8080 | 3.5893 |
| H | 0.3323 | 0.1947 | 0.9876 | 1.7261 | 1.3633 | 7.0456 | 1.7553 | 1.4353 | 7.2690 |
| H | 0.6677 | 0.8053 | 0.4876 | 2.0617 | 5.1973 | 3.4722 | 2.1649 | 5.3544 | 3.5913 |
| H | 0.1376 | 0.8053 | 0.9876 | −2.0617 | 5.1973 | 7.0456 | −2.1616 | 5.3544 | 7.2699 |
| H | 0.1376 | 0.3323 | 0.4876 | −0.3176 | 2.1765 | 3.4722 | −0.3603 | 2.2401 | 3.5893 |
| H | 0.6677 | −0.1376 | 0.9876 | 5.5318 | −0.8132 | 7.0456 | 5.7168 | −0.7994 | 7.2710 |
| H | 0.1947 | −0.1376 | 0.4876 | 2.0437 | −0.8132 | 3.4722 | 2.1220 | −0.7962 | 3.5891 |
| H | 0.1947 | 0.3323 | 0.9876 | 0.3176 | 2.1765 | 7.0456 | 0.3654 | 2.2377 | 7.2690 |
| H | 0.8053 | 0.6677 | 0.4876 | 3.4701 | 4.3841 | 3.4722 | 3.5546 | 4.5520 | 3.5913 |
| H | −0.1376 | 0.6677 | 0.9876 | −3.4701 | 4.3841 | 7.0456 | −3.5507 | 4.5511 | 7.2710 |
| H | −0.1376 | 0.1947 | 0.4876 | −1.7261 | 1.3633 | 3.4722 | −1.7506 | 1.4396 | 3.5891 |
| O | 0.3334 | 0.0000 | 0.0588 | 2.5209 | 0.0000 | 0.4469 | 2.6267 | 0.0076 | 0.4866 |
| O | 0.6666 | 0.0000 | 0.5588 | 5.0545 | 0.0000 | 4.0203 | 5.2088 | 0.0082 | 4.1658 |
| O | 0.6666 | 0.6666 | 0.0588 | 2.5273 | 4.3773 | 0.4469 | 2.6042 | 4.5106 | 0.4896 |
| O | 0.3334 | 0.3334 | 0.5588 | 1.2605 | 2.1832 | 4.0203 | 1.3131 | 2.2744 | 4.1662 |
| O | 0.0000 | 0.3334 | 0.0588 | −1.2605 | 2.1832 | 0.4469 | −1.3068 | 2.2786 | 0.4866 |
| O | 0.0000 | 0.6666 | 0.5588 | −2.5273 | 4.3773 | 4.0203 | −2.5973 | 4.5151 | 4.1658 |
| O | 0.6665 | 0.0000 | 0.9352 | 5.0438 | 0.0000 | 6.6999 | 5.2372 | 0.0031 | 6.9304 |
| O | 0.3335 | 0.0000 | 0.4352 | 2.5316 | 0.0000 | 3.1264 | 2.6021 | 0.0065 | 3.2497 |
| O | 0.3335 | 0.3335 | 0.9352 | 1.2658 | 2.1925 | 6.6999 | 1.3005 | 2.2525 | 6.9293 |
| O | 0.6665 | 0.6665 | 0.4352 | 2.5219 | 4.3681 | 3.1264 | 2.6193 | 4.5367 | 3.2524 |
| O | 0.0000 | 0.6665 | 0.9352 | −2.5219 | 4.3681 | 6.6999 | −2.6159 | 4.5371 | 6.9304 |
| O | 0.0000 | 0.3335 | 0.4352 | −1.2658 | 2.1925 | 3.1264 | −1.2954 | 2.2568 | 3.2497 |

## DIPOLE MOMENTS

Dipole moments (in Debye) of the water clusters as calculated by all the methods considered here along with available experimental values. Note that the dipole moment of the tetramer is zero by symmetry.

| Cluster | Exp. [1] | MP2 | vdW-DF | PBE | LDA |
|---|---|---|---|---|---|
| monomer | 1.855 | 1.859 | 1.86 | 1.8496 | 1.8774 |
| dimer | 2.643 | 2.6377 | 2.635 | 2.7103 | 2.7052 |
| trimer | — | 1.0802 | 1.0481 | 1.2039 | 1.2618 |
| tetramer | 0 | 0 | 0 | 0 | 0 |
| pentamer | — | 0.9891 | 0.96068 | 1.0581 | 1.1080 |

## VIBRATIONAL FREQUENCIES

### Monomer Frequencies in cm$^{-1}$

| LDA | PBE | vdW-DF | MP2 | Exp. [2] |
|---|---|---|---|---|
| 1532 | 1560 | 1586 | 1628 | 1595 |
| 3727 | 3765 | 3746 | 3822 | 3665 |
| 3854 | 3894 | 3866 | 3948 | 3760 |

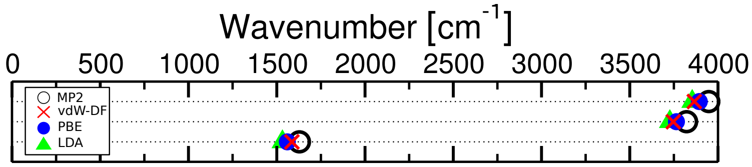


### Dimer Frequencies in cm$^{-1}$

| LDA | PBE | vdW-DF | MP2 | Exp. [2] |
|---|---|---|---|---|
| 453 | 378 | 358 | 344 | 309 |
| 784 | 661 | 555 | 608 | 522 |
| 1527 | 1563 | 1598 | 1629 | 1599 |
| 1556 | 1588 | 1612 | 1648 | 1616 |
| 3415 | 3585 | 3663 | 3727 | 3591 |
| 3712 | 3761 | 3746 | 3815 | 3661 |
| 3813 | 3856 | 3842 | 3917 | 3734 |
| 3835 | 3884 | 3863 | 3936 | 3763 |

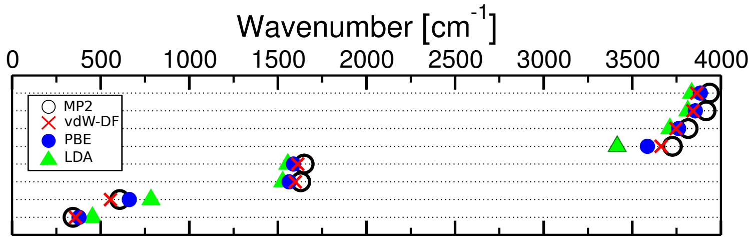

**Trimer Frequencies in $cm^{-1}$**

| LDA | PBE | vdW-DF | MP2 | Exp. [3] |
|---|---|---|---|---|
| 304 | 237 | 196 | 182 | — |
| 311 | 241 | 212 | 193 | — |
| 319 | 246 | 227 | 212 | — |
| 333 | 288 | 254 | 230 | — |
| 484 | 408 | 345 | 334 | 280 |
| 496 | 416 | 353 | 346 | 312 |
| 602 | 508 | 427 | 433 | 387 |
| 847 | 669 | 544 | 555 | 434 |
| 928 | 748 | 632 | 649 | 569 |
| 1193 | 984 | 814 | 833 | — |
| 1542 | 1578 | 1601 | 1638 | — |
| 1548 | 1581 | 1601 | 1641 | 1608 |
| 1595 | 1606 | 1622 | 1664 | — |
| 2838 | 3320 | 3536 | 3599 | 3472 |
| 3058 | 3420 | 3584 | 3656 | 3518 |
| 3068 | 3431 | 3595 | 3665 | 3530 |
| 3796 | 3845 | 3831 | 3904 | — |
| 3800 | 3847 | 3837 | 3907 | 3724 |
| 3802 | 3849 | 3838 | 3908 | 3726 |

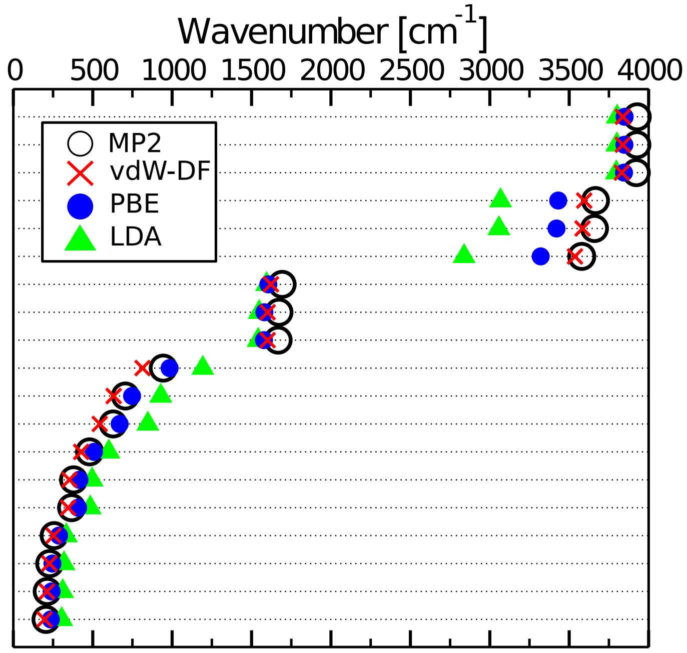

**Tetramer Frequencies in cm$^{-1}$**

| LDA | PBE | vdW-DF | MP2 |
|---|---|---|---|
| 295 | 232 | 194 | 201 |
| 301 | 256 | 213 | 205 |
| 333 | 282 | 235 | 229 |
| 333 | 282 | 235 | 229 |
| 395 | 299 | 259 | 245 |
| 404 | 299 | 272 | 245 |
| 404 | 306 | 272 | 250 |
| 414 | 343 | 298 | 278 |
| 520 | 463 | 399 | 394 |
| 588 | 504 | 426 | 421 |
| 588 | 514 | 448 | 436 |
| 589 | 514 | 448 | 436 |
| 1020 | 845 | 724 | 730 |
| 1144 | 940 | 790 | 793 |
| 1144 | 940 | 790 | 793 |
| 1327 | 1112 | 944 | 952 |
| 1528 | 1574 | 1600 | 1643 |
| 1562 | 1597 | 1615 | 1656 |
| 1562 | 1597 | 1615 | 1656 |
| 1620 | 1636 | 1641 | 1684 |
| 2277 | 3005 | 3339 | 3433 |
| 2630 | 3165 | 3424 | 3519 |
| 2630 | 3165 | 3424 | 3519 |
| 2742 | 3224 | 3459 | 3556 |
| 3797 | 3844 | 3827 | 3899 |
| 3797 | 3845 | 3828 | 3900 |
| 3797 | 3845 | 3828 | 3900 |
| 3797 | 3845 | 3829 | 3900 |

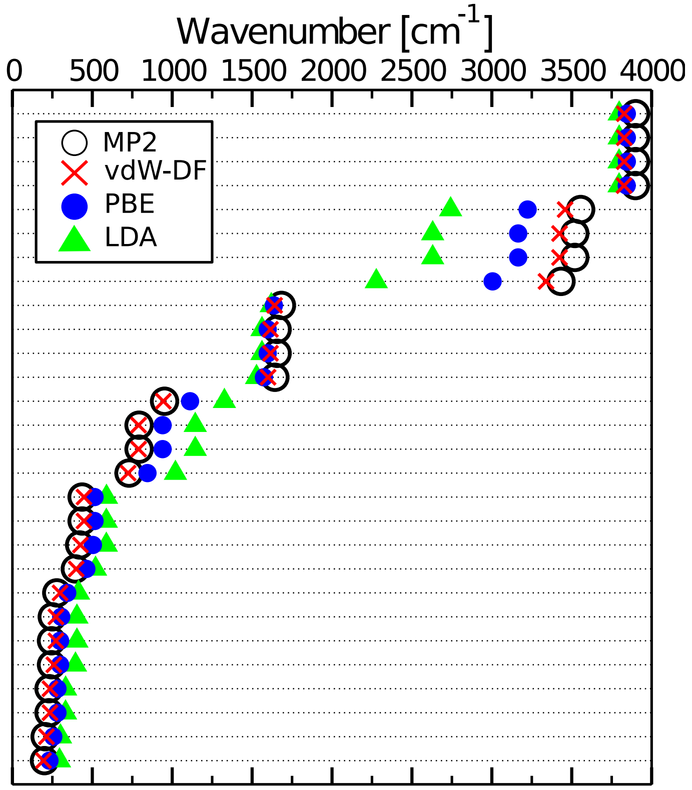

**Pentamer Frequencies in cm$^{-1}$**

| LDA | PBE | vdW-DF | MP2 |
|---|---|---|---|
| 313 | 272 | 224 | 215 |
| 353 | 277 | 232 | 225 |
| 386 | 284 | 258 | 231 |
| 393 | 319 | 271 | 251 |
| 402 | 339 | 292 | 280 |
| 490 | 352 | 297 | 287 |
| 493 | 361 | 300 | 290 |
| 538 | 479 | 408 | 402 |
| 548 | 491 | 420 | 418 |
| 593 | 522 | 445 | 437 |
| 608 | 532 | 457 | 450 |
| 684 | 606 | 529 | 506 |
| 979 | 816 | 687 | 692 |
| 1077 | 892 | 756 | 761 |
| 1178 | 976 | 823 | 827 |
| 1214 | 1005 | 846 | 847 |
| 1318 | 1105 | 937 | 943 |
| 1524 | 1578 | 1603 | 1646 |
| 1548 | 1593 | 1612 | 1656 |
| 1578 | 1611 | 1625 | 1666 |
| 1614 | 1634 | 1639 | 1682 |
| 1644 | 1649 | 1650 | 1690 |
| 2097 | 2921 | 3292 | 3396 |
| 2457 | 3070 | 3368 | 3470 |
| 2463 | 3079 | 3376 | 3479 |
| 2622 | 3156 | 3418 | 3521 |
| 2628 | 3165 | 3427 | 3530 |
| 3798 | 3846 | 3826 | 3897 |
| 3800 | 3847 | 3827 | 3899 |
| 3801 | 3848 | 3829 | 3901 |
| 3802 | 3850 | 3831 | 3902 |
| 3804 | 3851 | 3833 | 3903 |

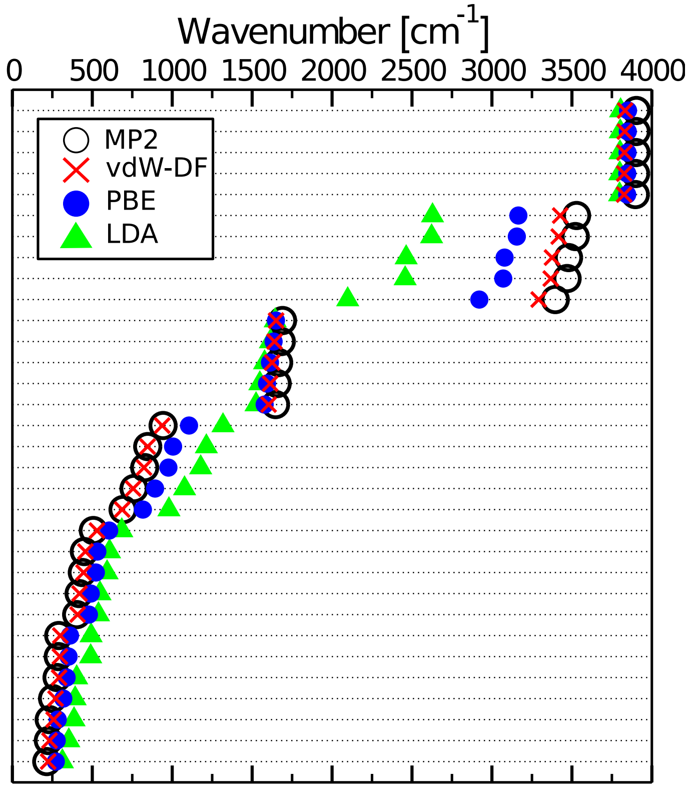

**Ice $I_h$ Frequencies in cm$^{-1}$**

Because of the size and complexity of the ice $I_h$ structure, MP2 calculations were not performed on it. All three DFT functionals were, however, used to calculate the vibrational frequencies of ice $I_h$. The results, presented here, exhibit trends similar to those seen in the small water clusters.

| LDA | PBE | vdW-DF | LDA | PBE | vdW-DF | LDA | PBE | vdW-DF |
|---|---|---|---|---|---|---|---|---|
| 277 | 209 | 205 | 1006 | 846 | 732 | 1630 | 1650 | 1648 |
| 281 | 212 | 208 | 1024 | 854 | 736 | 1633 | 1663 | 1662 |
| 299 | 226 | 208 | 1029 | 868 | 750 | 1655 | 1671 | 1667 |
| 304 | 231 | 214 | 1043 | 887 | 769 | 1668 | 1677 | 1668 |
| 345 | 262 | 236 | 1073 | 904 | 784 | 1671 | 1679 | 1672 |
| 348 | 263 | 248 | 1088 | 908 | 791 | 2146 | 2914 | 3190 |
| 350 | 268 | 253 | 1094 | 922 | 804 | 2177 | 2943 | 3216 |
| 351 | 271 | 263 | 1108 | 931 | 807 | 2203 | 2961 | 3229 |
| 394 | 286 | 266 | 1123 | 941 | 823 | 2212 | 2969 | 3232 |
| 411 | 297 | 281 | 1165 | 981 | 862 | 2221 | 2975 | 3244 |
| 425 | 318 | 288 | 1167 | 987 | 867 | 2224 | 2984 | 3254 |
| 449 | 332 | 306 | 1182 | 1011 | 889 | 2224 | 2984 | 3255 |
| 489 | 359 | 311 | 1194 | 1020 | 896 | 2233 | 2989 | 3256 |
| 492 | 360 | 318 | 1212 | 1022 | 900 | 2260 | 3026 | 3299 |
| 494 | 363 | 323 | 1217 | 1029 | 900 | 2271 | 3033 | 3306 |
| 502 | 368 | 331 | 1262 | 1072 | 949 | 2272 | 3034 | 3309 |
| 519 | 383 | 343 | 1277 | 1084 | 960 | 2336 | 3061 | 3323 |
| 788 | 658 | 557 | 1309 | 1103 | 970 | 2360 | 3065 | 3325 |
| 808 | 678 | 573 | 1313 | 1110 | 978 | 2685 | 3187 | 3372 |
| 815 | 682 | 574 | 1339 | 1138 | 1007 | 2725 | 3194 | 3373 |
| 816 | 684 | 576 | 1343 | 1146 | 1013 | 2725 | 3195 | 3375 |
| 853 | 721 | 612 | 1373 | 1168 | 1039 | 2766 | 3241 | 3423 |
| 863 | 734 | 630 | 1410 | 1192 | 1057 | 2776 | 3248 | 3429 |
| 907 | 750 | 636 | 1550 | 1608 | 1618 | 2800 | 3256 | 3433 |
| 926 | 763 | 648 | 1572 | 1613 | 1621 | 2804 | 3261 | 3434 |
| 951 | 803 | 692 | 1573 | 1613 | 1621 | 2808 | 3264 | 3436 |
| 959 | 812 | 701 | 1579 | 1615 | 1622 | 2812 | 3265 | 3443 |
| 970 | 813 | 708 | 1586 | 1615 | 1625 | 2840 | 3268 | 3445 |
| 1002 | 825 | 709 | 1615 | 1636 | 1633 | 2859 | 3270 | 3448 |
| 1003 | 832 | 721 | 1618 | 1646 | 1645 | | | |

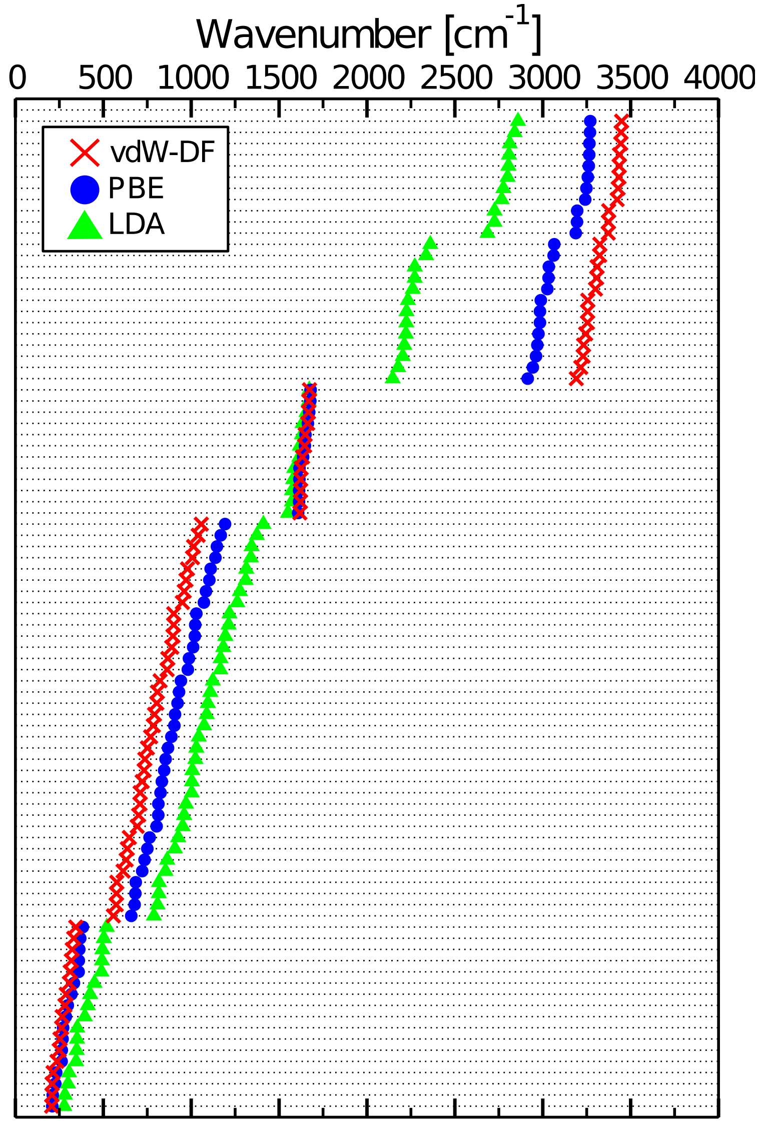


[1] J. K. Gregory, D. C. Clary, K. Liu, M. G. Brown, and R. J. Saykally, Science **275**, 814 (1997).
[2] J. Ceponkus, P. Uvdal, and B. Nelander, J. Chem. Phys. **129**, 194306 (2008).
[3] B. Tremblay, B. Madebène, M. E. Alikhani, and J. P. Perchard, Chem. Phys. **378**, 27 (2010).
